# Supplementary material for: Refractive Geometry for Underwater Domes
Source: arXiv:2108.06575 source file (2021-09-28)

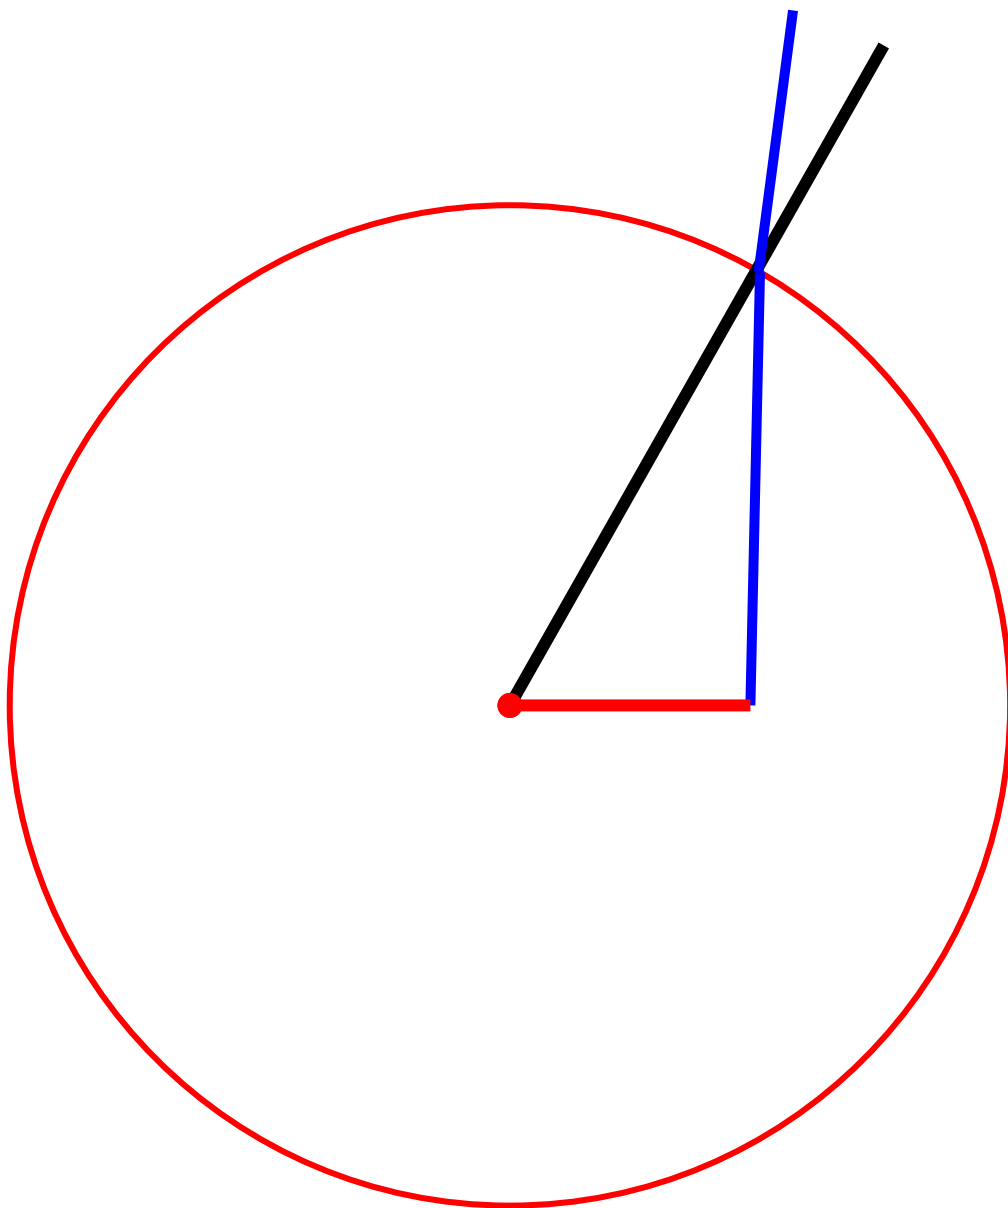

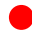

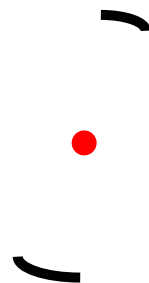

Supplement: Supplementary file 1 [file SupplementalMaterial.pdf]
